# Supplementary material for: DTGAN: Differential Private Training for Tabular GANs
Source: arXiv:2107.02521 source file (2021-08-02)
Supplement: Supplementary file 1 [file appendix.tex]

\chapter{Differential Privacy Experimental Setup}

The supplementary material highlights the network architecture shared between PATE-GAN~\cite{pategan} and DP-WGAN~\cite{xie2018differentially} as mentioned in~Sec.~\ref{Ch5:ES}. Additionally, it provides hyper-parameters used for conducting the data utility (i.e., statistical similarity $\&$ ML utility) as well as the membership and attribute inference attack experiments.

\section{Network Architecture}
\label{appendix:1}

The network architecture for training PATE-GAN is used identically to their original implementation provided on github\footnote{\url{https://github.com/vanderschaarlab/mlforhealthlabpub/tree/main/alg/pategan}}. And, the network structure of DP-WGAN\footnote{\url{https://github.com/BorealisAI/private-data-generation/blob/master/models/dp_wgan.py}} used in the experiments has been modified from the original to have the exact neural network architecture for the discriminator and generator networks as that of PATE-GAN. This is done to study the performance of DP-WGAN in relation to PATE-GAN.

The generator network of PATE-GAN comprises of a shallow neural network with 3 fully connected layers that each comprise of $4*l$ nodes where $l$ is the length of each row in the original data. The first 2 fully connected layers are followed by a \textit{Tanh activation} whereas for the last layer a \textit{Sigmoid activation} is used. This is done to bring the values generated in the range of [0,1] which is the same range as the normalised data used for training. 

The student discriminator network of PATE-GAN comprises of a shallow neural network with 2 fully connected layers with $l$ nodes. The first layer is followed by a \textit{ReLU activation function} whereas the output of the second layer is used directly for computing the KL divergence loss of the discriminator as shown in Eq.~\ref{eq:gan}. 

\section{Network Hyper-parameters}
\label{appendix:2}

Across all baselines, the batch size was set to 64. Moreover, for PATE-GAN and DP-WGAN, default hyper-parameters as found in the code-bases were utilized. Thus, PATE-GAN uses 10 as the default number of teacher discriminators for all experiments. And DP-WGAN, uses [-0.01,0.01] to clamp the weights of the discriminator and $0.1$ as the gradient norm bound $C$.   

Additionally, Tab.~\ref{tab:app0} and Tab.~\ref{tab:app1} provide details concerning the differential-private hyper-parameters such as the noise scale used and the number of training epochs\footnote{Note that in the original implementation of PATE-GAN, the privacy budget $\epsilon=1$ is expended with just one iteration over a single batch. Therefore, in the epochs columns, the number of iterations over a single batch is displayed.} required for generating synthetic tabular data with the corresponding privacy budget epsilon (i.e., $\epsilon$) to conduct the data utility experiments and privacy attack experiments in Sec.~\ref{Ch5:ES}.

\begin{table}[htb]
\centering
\caption{\centering Differential privacy hyper-parameters for conducting statistical similarity and ML utility experiments.}
\resizebox{0.8\columnwidth}{!}{
\begin{tabular}{|c|c|c|c|c|c|}
\hline
\textbf{Model}  & \textbf{Dataset} & \textbf{No. of Discriminators} & \textbf{Noise Scale} & \textbf{Epochs} & \textbf{Epsilon} \\
\hline
PATE-GAN     & Adult   & 1                        & 1           & 1      & 1       \\
PATE-GAN     & Credit  & 1                        & 1           & 1      & 1       \\
PATE-GAN     & Loan    & 1                        & 1           & 1      & 1       \\
DP-WGAN      & Adult   & 1                        & 1.012       & 1      & 1       \\
DP-WGAN      & Credit  & 1                        & 1.012       & 1      & 1       \\
DP-WGAN      & Loan    & 1                        & 1.33        & 1      & 1       \\
D-DP-CTABGAN & Adult   & 1                        & 1.06        & 1      & 1       \\
D-DP-CTABGAN & Credit  & 1                        & 1.06        & 1      & 1       \\
D-DP-CTABGAN & Loan    & 1                        & 1.58        & 1      & 1       \\
G-DP-CTABGAN & Adult   & 1000                     & 3.518       & 1      & 1       \\
G-DP-CTABGAN & Credit  & 1000                     & 3.53        & 1      & 1       \\
G-DP-CTABGAN & Loan    & 1000                     & 1.28        & 1      & 1       \\
PATE-GAN     & Adult   & 1                        & 1           & 795    & 100     \\
PATE-GAN     & Credit  & 1                        & 1           & 795    & 100     \\
PATE-GAN     & Loan    & 1                        & 1           & 795    & 100     \\
DP-WGAN      & Adult   & 1                        & 0.33        & 6      & 100     \\
DP-WGAN      & Credit  & 1                        & 0.33        & 6      & 100     \\
DP-WGAN      & Loan    & 1                        & 0.38        & 7      & 100     \\
D-DP-CTABGAN & Adult   & 1                        & 0.36        & 5      & 100     \\
D-DP-CTABGAN & Credit  & 1                        & 0.36        & 5      & 100     \\
D-DP-CTABGAN & Loan    & 1                        & 0.42        & 4      & 100     \\
G-DP-CTABGAN & Adult   & 50                       & 0.867       & 1      & 100     \\
G-DP-CTABGAN & Credit  & 100                      & 0.874       & 1      & 100     \\
G-DP-CTABGAN & Loan    & 100                      & 1.089       & 4      & 100    \\
\hline
\end{tabular}
}
\label{tab:app0}
\end{table}

\begin{table}[htb]
\centering
\caption{\centering Differential privacy hyper-parameters for conducting membership and attribute inference attacks.}
\resizebox{0.8\columnwidth}{!}{
\begin{tabular}{|c|c|c|c|c|c|c|}
\hline
\textbf{Model} & \textbf{Dataset} & \textbf{No of Discriminators} & \textbf{Noise Scale (Membership)} & \textbf{Noise Scale (Attribute)} & \textbf{Epochs} & \textbf{Epsilon} \\ \hline
PATE-GAN     & Adult  & 1    & 1    & 1    & 1 & 1 \\
PATE-GAN     & Credit & 1    & 1    & 1    & 1 & 1 \\
PATE-GAN     & Loan   & 1    & 1    & 1    & 1 & 1 \\
DP-WGAN      & Adult  & 1    & 1.33 & 1.25 & 1 & 1 \\
DP-WGAN      & Credit & 1    & 1.33 & 1.25 & 1 & 1 \\
DP-WGAN      & Loan   & 1    & 1.33 & 1.25 & 1 & 1 \\
D-DP-CTABGAN & Adult  & 1    & 1.67 & 1.56 & 1 & 1 \\
D-DP-CTABGAN & Credit & 1    & 1.67 & 1.56 & 1 & 1 \\
D-DP-CTABGAN & Loan   & 1    & 1.67 & 1.56 & 1 & 1 \\
G-DP-CTABGAN & Adult  & 1000 & 1.28 & 1.37 & 1 & 1 \\
G-DP-CTABGAN & Credit & 1000 & 1.28 & 1.37 & 1 & 1 \\
G-DP-CTABGAN & Loan   & 1000 & 1.28 & 1.37 & 1 & 1 \\
\hline
\end{tabular}
}
\label{tab:app1}
\end{table}
